# Supplementary material for: Prediction with a Short Memory
Source: arXiv:1612.02526 source file (2018-06-28)
Supplement: Supplementary file 7 [file hmm_appendix_old.tex]

\section{Proof of High Probability Guarantees for HMMs}\label{sec:hmm_app}

%We also show that the dependence on $c$ is optimal in Corollary \ref{0/1}. Consider a permutation on $n$ states, with the outputs being binary. Label each state with `+' or `-', the states labeled as `+' emit 1 with probability $0.5+1/c$ and the states labeled as `-' emit 0 with probability $0.5+1/c$. Consider the task of distinguishing a sequence $s_1$ of $\log n$ `+' states from a sequence $s_2$  with $\log n/2$ `+' states and $\log n/2$ `-' states. The expected number of 1 for sequence $s_1$ is 

\hmmwhp*
\begin{proof}
	
	Define $\gamma=1/\epsilon$. Recall that the Markov model with knowledge of the true distribution of the data that predicts based on the past $\ell$ observations corresponds exactly to the Bayes optimal predictor that has knowledge of the true HMM but only observes the most recent $\ell$ observations. Without loss of generality, let the predictions start from time 0. We will compare the prediction of the $\ell$-th order Markov model $\mathcal{P}_{\ell}$ with an oracle $\mathcal{O}$ which knows the hidden state at time 0, and then relate to the error with respect to $\mathcal{P}_{\infty}$ using the triangle inequality. Consider the modified $\ell$-th order predictor $\mathcal{P}'_{\ell}$ which only has access to outputs from time 0 to $(t-1)$ when making the predictions at time $t$, for $t \le \ell$. By Lemma \ref{longer_is_better} the performance of $\mathcal{P}_{\ell}$ is at most a factor of two worse than the performance of $\mathcal{P}'_{\ell}$, hence we will upper bound the average error of the predictor $\mathcal{P}'_{\ell}$.
	
	\begin{restatable}{lemma}{longerisbetter}\label{longer_is_better}
		If the average $\ell_1$ prediction error of the Markov model of order $l_1$ is $\epsilon$, then the average  $\ell_1$ prediction error of the Markov model of order $l_2$ where $l_2>l_1$ is at most $2\epsilon$.
	\end{restatable}
	
	Without loss of generality, let the true hidden state at time 0 be 1. We refer to the hidden state at time at by $h_t$ and the output at time $t$ by $x_t$. Let $z_{i,t} (s_0^t)=\Pr[h_0 = i | x_0^t = s_0^t]$ be the posterior probability of the $i$th hidden state after seeing the observations $s_0^t$ up to time $t$. We refer to $z_{1,t} (s_0^t)$ by $u_t (s_0^t)$. Also let $v_t (s_0^t)=\sum_{i=2}^{n}z_{i,t} (s_0^t)=1-u_t (s_0^t)$ be the sum of the posterior probabilities of all the remaining states. Let $\{z'_{i,t} (s_0^t)=z_{i,t} (s_0^t)/v_t (s_0^t), \forall \; i \ne 1\}$ be the conditional posterior probability of the $i$th hidden state conditioned on the starting state not being 1 and seeing the outputs $s_0^t$. Let $p_{i,j}^{t+1} (s_0^t)=\Pr[y[t+1]=j|x_0^t = s_0^t, h_0=i]$ be the probability of seeing output $j$ at time $t+1$ conditioned on $h_0=i$ and seeing the outputs $s_0^t$. We refer to $p_{1,j}^{t+1}(s_0^t)$ by just $p_j^{t+1}(s_0^t)$ for notational ease. We also refer to the distribution $\{p_j^{t+1}(s_0^t), j \in [d]\}$ by $p^{t+1}(s_0^t)$. Define the predictive distribution of the predictor $\mathcal{P}'_{\ell}$ as $\{b_{j}^{t+1} (s_0^t)=\Pr[y[t+1]=j|x_0^t = s_0^t], j\in [d]\}$.  Also define the output distribution at time $t+1$ conditioned on the starting distribution $\{z'_{i,t}(s_0^t), i \ne 1\}$ and seeing the outputs $s_0^t$ be $q^{t+1}(s_0^t)$. Let the $\ell_1$ distance between the predictive distributions of the oracle and the predictor $\mathcal{P}'_{\ell}$ at the $(t+1)$th step on seeing the outputs $s_0^t$ be $\delta_{t+1} (s_0^t)$. Hence $\delta_{t+1} (s_0^t)=\parallel(p^{t+1}(s_0^t) - b_{j}^{t+1} (s_0^t)\parallel_1$.
	
	Our proof relies on a martingale concentration argument, and in order to ensure that our martingale has bounded differences we will ignore outputs which cause a significant drop in the posterior of the true hidden state at time 0. Let $B$ be the set of all outputs $j$ at some time $t$ such that $\frac{p_j^{t+1}(s_0^t)}{q_j^{t+1}(s_0^t)} \le \frac{1}{c\gamma^4{\log n}}$. Note that, $\sum_{j\in B}^{}p_j^{t+1}(s_0^t) \le \frac{\sum_{j\in B}^{}q_j^{t+1}(s_0^t)}{c\gamma^4{\log n}}\le \frac{1}{c\gamma^4{\log n}}$. Hence by a union bound, with failure probability at most $1/\gamma^2$ any output $j$ such that $\frac{p_j^{t+1}(s_0^t)}{q_j^{t+1}(s_0^t)} \le \frac{1}{c\gamma^4{\log n}}$ is not emitted in a window of length $c\gamma^2{\log n}$. Hence we will only argue about sequences of outputs such that the output $j$ emitted at each step satisfies $\frac{p_j^{t+1}(s_0^t)}{q_j^{t+1}(s_0^t)} \ge \frac{1}{c\gamma^4{\log n}}$, the contribution of all the remaining sequences to the error is at most $1/\gamma^2$, let the set of all such outputs be $\mathcal{S}_1$. Let $\E_{\mathcal{S}_1}[X]$ be the expectation of any random variable $X$ conditioned on the output sequence being in the set $\mathcal{S}_1$.
	
	Consider the sequence of random variables $X_t  (s_0^t)= \log u_t  (s_0^t)- \log v_t (s_0^t)$. Let $\Delta_{t+1}(s_0^t,j)= X_{t+1}  (s_0^{t+1})- X_t  (s_0^t)$ be the change in $X_t  (s_0^t)$ on seeing the  output $j$ at time $t+1$. We will first find an expression for $\Delta_{t+1}(j)$. The posterior probabilities after seeing the $(t+1)$th output get updated according to Bayes rule--
	\begin{align}
	\Pr[h_0 = 1 | x_0^t = s_0^t, x[t+1]=j] &= \frac{\Pr[h_0 = 1 | x_0^t = s_0^t]\Pr[x[t+1] = j | h_0 = 1, x_0^t = s_0^t]}{\Pr[x[t+1] = j |x_0^t = s_0^t]}\nonumber\\
	\implies u_{t+1}(s_0^{t+1}) &= \frac{u_t(s_0^t)p_j^{t+1}(s_0^t)}{\Pr[x[t+1] = j |x_0^t = s_0^t]}\nonumber
	\end{align}
	Let $\Pr[x[t+1] = j |x_0^t = s_0^t]=c_j(s_0^t)$. Note that $z_{i,t+1}(s_0^{t+1})=z_{i,t}(s_0^t)p_{i,j}^{t+1}(s_0^t)/c_j(s_0^t)$ if the output at time $t+1$ is $j$. We can write--
	\begin{align}
	q_j^{t+1}(s_0^t)&=\Big({\sum_{i=2}^{k}z_{i,t}p_{i,j}^{t+1}(s_0^t)}\Big)/{v_t(s_0^t)} \nonumber\\ 
	v_{t+1}(s_0^{t+1}) &= \sum_{i=2}^{k}z_{i,t+1}(s_0^{t+1})=\Big(\sum_{i=2}^{k}z_{i,t}(s_0^t)p_{i,j}^{t+1}(s_0^t)\Big)/c_j(s_0^t) \nonumber\\
	&= v_t(s_0^t)q_j^{t+1}(s_0^t)/c_j(s_0^t)\nonumber
	\end{align}
	Therefore we can write $\Delta_{t+1}(s_0^t,j)$ and its expectation $\E[\Delta_{t+1}(s_0^t)]$ as--
	\begin{align}
	\Delta_{t+1}(s_0^t,j) &= \log \frac{p_j^{t+1}(s_0^t)}{q_j^{t+1}(s_0^t)}\nonumber \\
	\implies \E[\Delta_{t+1,j}(s_0^t)] &= \sum_{j}^{}p_j^{t+1}(s_0^t)\log \frac{p_j^{t+1}(s_0^t)}{q_j^{t+1}(s_0^t)} = D(p_j^{t+1}(s_0^t) \parallel q_j^{t+1}(s_0^t)) \nonumber
	\end{align}
	We define a truncated version of $\Delta_{t+1}(s_0^t,j)$ to keep martingale differences bounded. 
	\[ \tilde{\Delta}_{t+1}(j) =\begin{cases} 
	\Delta_{t+1}(s_0^t,j) & \frac{p_j^{t+1}(s_0^t)}{q_j^{t+1}(s_0^t)}\le {\log n} \\
	\log({\log n})& \frac{p_j^{t+1}(s_0^t)}{q_j^{t+1}(s_0^t)}> {\log n}
	\end{cases}
	\]
	$\E[\tilde{\Delta}_{t+1}(s_0^t)]$ then equals a truncated version of the KL-divergence which we define as follows.
	\begin{definition}\label{cool_Kl}
		For any two distributions $\mu(x)$ and $\nu(x)$, define the truncated KL-divergence as $\tilde{D}_C(\mu\parallel \nu) = \E[\log (\max\{\mu(x)/\nu(x),C\})] $ for some fixed $C$.
	\end{definition}
	We are now ready to define our martingale. Consider the sequence of random variables $\tilde{X}_t(s_0^t) = \tilde{X}_{t-1}(s_0^{t-1}) + \tilde{\Delta}_t(s_0^t)$ and define  $\tilde{Z}_t(s_0^t) = \sum_{t=1}^{n}\Big(\tilde{X}_t(s_0^t) - \tilde{X}_{t-1}(s_0^{t-1}) -\delta_{t}(s_0^t)^2/2\Big)$. Note that $\Delta(s_0^t) \ge \tilde{\Delta}(s_0^t) \implies X_t(s_0^t) \ge \tilde{X}_t(s_0^t)$. 
	
	\begin{lemma}
		$\E_{\mathcal{S}_1}[\tilde{X}_{t+1} (s_0^{t+1})-\tilde{X}_{t} (s_0^t)] \ge \delta_{t+1} (s_0^t)^2/2$, where the expectation is with respect to the output at time $t+1$. Hence the sequence of random variables $\tilde{Z}_t(s_0^t) = \sum_{i=1}^{n}\Big(\tilde{X}_t(s_0^t)-\tilde{X}_{t-1}(s_0^{t-1})-\delta_{t}(s_0^t)^2/2\Big)$ is a submartingale with respect to the outputs.
	\end{lemma}
	\begin{proof}
		By definition $\tilde{X}_t(s_0^t) - \tilde{X}_{t-1}(s_0^{t-1}) = \tilde{\Delta}_t(s_0^t)$ and $\E[\tilde{\Delta}_t(s_0^t)] = \tilde{D}_{C}(p_j^{t+1}(s_0^t) \parallel q_j^{t+1}(s_0^t)), C= {\log n}$. As the expectation is only over sequences in $\mathcal{S}_1$, hence we are only removing events which have a negative contribution to ${\tilde{D}_{C}(p_j^{t+1}(s_0^t) \parallel q_j^{t+1}(s_0^t))}$, hence $$\E_{\mathcal{S}_1}[\tilde{X}_{t+1} (s_0^{t+1})-\tilde{X}_{t} (s_0^t)] \ge {\tilde{D}_{C}(p_j^{t+1}(s_0^t) \parallel q_j^{t+1}(s_0^t))}$$. We can now apply Lemma \ref{cool_pinsker}. 
		\coolKL
		Hence $\E_{\mathcal{S}_1}[\tilde{\Delta}_t(s_0^t)] \ge \frac{1}{2}\norm{p^{t+1}(s_0^t)-q^{t+1}(s_0^t)}{1}^2$. Note that the predictive distribution $b^{t+1}(s_0^t)$ of the predictor $\mathcal{P}'_{\ell}$ is a convex combination of $p^{t+1}(s_0^t)$ and $q^{t+1}(s_0^t)$ and equals $b^{t+1}=u_t(s_0^t) p^{t+1} + v_t(s_0^t) q^{t+1}(s_0^t)$. Therefore ${\norm{p^{t+1}(s_0^t)-q^{t+1}(s_0^t)}{1}^2} \ge {\norm{p^{t+1}(s_0^t)-b^{t+1}(s_0^t)}{1}^2} = \delta_{t+1} (s_0^t)^2 $ hence $\E_{\mathcal{S}_1}[\tilde{X}_{t+1} (s_0^{t+1})-\tilde{X}_{t} ]\ge \delta_{t+1} (s_0^t)^2/2$. 
	\end{proof}
	
	\begin{comment}
	In order to get a good upper bound on the submartingale, we make a small modification to it. Once $y_t$ goes down below $1/n^2$ we cap it at $1/n^2$ and fix it at $\frac{1}{n^2}$ for making the remaining predictions in the window. We also correspondingly cap $x_t$ and fix it at $1-\frac{1}{n^2}$. Define $X'_t = \log x'_t - \log y'_t$, where $y'_t$ and $x'_t$ are the capped versions of $x_t$ and $y_t$. Also, define $\epsilon'_{t} = \{ \epsilon_t \;\text{if} \;\epsilon_t \ge \frac{1}{n}\; \text{and 0 otw}\}$. We prove that the new sequence of random variable $Z'_t = \sum_{i=1}^{t}(X'_t-X'_{t-1}-{\epsilon'_{t}}^2/2)$ is also a submartingale with respect to the outputs.
	
	\begin{lemma}
	$\E[X'_{t+1}-X'_{t}] \ge {\epsilon'_{t+1}}^2/2$, where the expectation is with respect to the output at time $t+1$. Hence the sequence of random variables $Z'_t$ is a submartingale with respect to the outputs.
	\end{lemma}
	\begin{proof}
	Note that $\E[X'_{t+1}-X'_{t}] \ge 0$, as $p\log x+ (1-p)\log (1-x)$ is maximized at $x=p$. Also, note that 
	\end{proof}
	\end{comment}
	
	We now claim that our submartingale has bounded differences.
	
	\begin{lemma}
		$|\tilde{Z}_{t+1}(s_0^{t+1})-\tilde{Z}_t(s_0^t)|\le \sqrt{2}\log (c\gamma^4{\log n})$.
	\end{lemma}
	\begin{proof}
		Note that $(\delta_{t+1}(s_0^{t+1})^2-\delta_t(s_0^t)^2)/2$ can be at most 1. $Z_{t+1}(s_0^{t+1})-Z_t(s_0^t) = \log (\tilde{\Delta}_j(s_0^t))$ where $j$ is the output at time $t+1$. By definition $\tilde{\Delta}_j(s_0^t) \le \log( {\log n})$. Also, $\tilde{\Delta}_j(s_0^t) \ge -\log(c\gamma^4 {\log n})$ as we only consider sequences with the property that at each step the output $j$ satisfies $\frac{p_j^{t+1}(s_0^t)}{q_j^{t+1}(s_0^t)} \ge \frac{1}{c\gamma^4{\log n}}$. Hence $|\tilde{Z}_{t+1}(s_0^{t+1})-\tilde{Z}_t(s_0^t)|\le \log (c\gamma^4{\log n}) + 1\le \sqrt{2}\log (c\gamma^4{\log n})$. 
	\end{proof}
	
	We now apply Azuma-Hoeffding --
	%\textbf{Azuma-Hoeffding inequality- }
	%\emph{
	%	Let $Z_i$ be a submartingale and let $|Z_{i}-Z_{i-1}|\le c$. Then $\Pr[Z_t-Z_0\le -\lambda] \le \exp\Big(\frac{-\lambda^2}{2tc^2}\Big)$
	%}
	\begin{lemma}\label{azuma}
		({Azuma-Hoeffding inequality}) Let $Z_i$ be a submartingale with $|Z_{i}-Z_{i-1}|\le M$. Then $\Pr[Z_t-Z_0\le -\lambda] \le \exp\Big(\frac{-\lambda^2}{2tM^2}\Big)$
	\end{lemma}
	Applying Lemma \ref{azuma} we can show,
	\begin{align}
	\Pr[\tilde{Z}_{\ell}(s_0^{\ell-1})-\tilde{Z}_0&\le -{\log n}] \le \exp\Big(\frac{-{\log n}}{4c\gamma^2\log^2(c\gamma^4{\log n})}\Big) \le 1/\gamma^2 \label{eq:azuma_app}
	\end{align}
	
	We now bound the average error in the window 0 to $\ell-1$. With failure probability at most $1/\gamma^2$ over the randomness in the outputs, $\tilde{Z}_{\ell}(s_0^{\ell-1})-\tilde{Z}_0\ge -{\log n}$ by Eq. \ref{eq:azuma_app}. Let $\mathcal{S}_2$ be the set of all sequences in $\mathcal{S}_1$ which satisfy $\tilde{Z}_{\ell}(s_0^{\ell-1})-\tilde{Z}_0\ge -{\log n}$. Note that $X_0 = \tilde{X}_0 \ge \log(1/\pi_i)$. Consider the last point after which $v_t(s_0^t)$ decreases below $1/\gamma^2$ and remains below that for every subsequent step in the window. Let this point be $\tau(s_0^{\ell-1})$, if there is no such point define $\tau(s_0^{\ell-1})$ to be $\ell-1$. The total contribution of the error at every step after the $\tau$th step to the average error is a $1/\gamma^2$ term as the error after this step is $1/\gamma^2$. Note that $X_{\tau}(s_0^{\tau}) \le \log \gamma^2 \implies \tilde{X}_{\tau}(s_0^{\tau}) \le \log \gamma^2$ as $X_{t}(s_0^{t}) \ge \tilde{X}_{t}(s_0^{t})$. Hence for all $s_0^{\ell-1}$ in $\mathcal{S}_2$--
	\begin{align}
	\tilde{X}_\tau(s_0^{\tau}) &\le \log \gamma^2 \nonumber \\
	\implies \tilde{X}_{\tau}(s_0^{\tau})  - \tilde{X}_0 &\le \log \gamma^2+\log(1/\pi_i)\nonumber\\
	\implies 0.5\sum_{t=0}^{\tau(s_0^{\ell})}{\delta}_{t}^2(s_0^{t-1})  &\le \log \gamma^2+\log(1/\pi_i) + {\log n} &(\text{By Eq. \ref{eq:azuma_app}})\nonumber\\
	%\implies \sum_{t=1}^{L}\epsilon_t(s_0^t)^2 &\le 4\log n + o(1)\\
	\implies \frac{\sum_{t=0}^{\ell-1}{\delta}_{t}^2(s_0^{t-1})}{c\gamma^2H} &\le 3/\gamma^2 &(\text{as } \log(1/\pi_i)\le c\log n)\nonumber \\
	\implies \delta_{\ell_1}(\mathcal{P}_{\ell}') &\le 2/\gamma &(\text{By Jensen's inequality}) \nonumber
	\end{align}
	Hence the predictor $\mathcal{P}'_L$ has average $\ell_1$ error at most $2/\gamma=2\epsilon$ with respect to $\mathcal{O}$. Therefore the predictor $\mathcal{P}_{\ell}$ has average $\ell_1$ error at most $4\epsilon$ with respect to $\mathcal{O}$. Also, by Lemma \ref{longer_is_better}, $P_{\infty} $ has average $\ell_1$ error at most $4 \epsilon$ with respect to $\mathcal{O}$. Using the triangle inequality, the predictor $\mathcal{P}_{\ell}$ has average $\ell_1$ error at most $8\epsilon$ with respect to $P_{\infty} $.
\end{proof}

\subsection{Proof of Lemma \ref{longer_is_better}}

\longerisbetter*
\begin{proof}
	Note that the optimal prediction over windows of length $l_2>l_1$ cannot be worse than the optimal prediction over windows of length $l_1$. Hence if the average prediction error of the Markov model of order $l_1$ is $\epsilon$, then the optimal error over windows of length $l_2$ is at most $\epsilon$. We claim that the prediction of the Markov model is at most a factor of 2 off the optimal.\\
	
	To verify, note that the optimal prediction $p_{\text{opt}}^{t+1}(s_0^t)$ to minimize $\ell_1$ loss given the posterior $\Pr[h_0|s_{0}^t]$ of the hidden state at time 0 given observations from time $0$ to $t$ is the median of the predictive distributions $p_{i}^{t+1}(s_0^t)$ of the hidden states $i$, weighted by the posterior probability $\Pr[h_0=i|s_{0^t}]=z_{i,t}(s_0^t)$. The predictive distribution of the Markov model equals $b^{t+1}(s_0^t)=\sum_i p_{i}^{t+1}(s_0^t)z_{i,l}(s_0^t)$ and is the mean of the predictive distributions. The $\ell_1$ loss of the Markov model equals $\sum_{j}^{}|b_j^{l+1}(s_0^l)-p_{j}^{l+1}(s_0^l)|$ whereas the $\ell_1$ loss of the optimal predictor equals $\sum_{j}^{}|p_{\text{opt},j}^{l+1}(s_0^l)-p_{j}^{l+1}(s_0^l)|$. By Lemma \ref{mean_median} $|b_j^{l+1}(s_0^l)-p_{j}^{l+1}(s_0^l)|\le 2|p_{\text{opt},j}^{l+1}(s_0^l)-p_{j}^{l+1}(s_0^l)|$. Hence $\sum_{j}^{}|b_j^{l+1}(s_0^l)-p_{j}^{l+1}(s_0^l)| \le 2\sum_{j}^{}|p_{\text{opt},j}^{l+1}(s_0^l)-p_{j}^{l+1}(s_0^l)|$. 
	
	\begin{lemma}\label{mean_median}
		For any distribution $\mu$, the expected deviation from the mean $\bar{x}$ is at most twice the expected deviation from the median $\tilde{x}$.
	\end{lemma}
	\begin{proof}
		Let the expected deviation from the median be $\delta$. We claim that $|\bar{x}-\tilde{x}|\le \delta$. To verify, note that
		\begin{align}
		|\bar{x}-\tilde{x}| &= \Big|\sum_{x}^{}\mu(x)(x-\tilde{x})\Big|\le \sum_{x}^{}\Big|\mu(x)(x-\tilde{x})\Big|\le \delta \nonumber
		\end{align}
		Hence by the triangle inequality--
		\begin{align}
		\sum_{x}^{}\mu(x)|x-\bar{x}| &\le \sum_{x}^{}\mu(x)|x-\tilde{x}| + \sum_{x}^{}\mu(x)|\tilde{x}-\bar{x}|\le 2\delta  \nonumber
		\end{align}
	\end{proof}
\end{proof}

\subsection{Proof of Lemma \ref{cool_pinsker}}

\coolKL*
\begin{proof}
	We rely on the following Lemma which bounds the KL-divergence for binary distributions-
	\begin{lemma}
		For every $0 \le q \le p\le 1$, we have
		\begin{enumerate}
			\item $p\log \frac{p}{q} + (1-p)\log \frac{1-p}{1-q} \ge 2(p-q)^2$
			\item $3p + (1-p)\log \frac{1-p}{1-q} \ge 2(p-q)^2$
		\end{enumerate}
	\end{lemma}
	\begin{proof}
		For the second result, first observe that $\log(1/(1-q))\ge 0$ and $(p-q)\le p$ as $q\le p$. Both the results then follow from standard calculus.
	\end{proof}
	Let $A := \{x \in X : \mu(x) \ge \nu(x)\}$ and $B := \{x \in X : \mu(x) \ge C\nu(x)\}$. Let $\mu(A)=p$, $\mu(B)=\delta,  \nu(A)=q$ and $\nu(B)=\epsilon$. Note that $\norm{\mu-\nu}{1}=2(\mu(A)-\nu(A))$. By the log-sum inequality--
	\begin{comment}
	\begin{align}
	D(\mu \parallel \nu) &= \sum_{x\in A}\mu(x)\log\frac{\mu(x)}{\nu(x)} + \sum_{x\in X-A}\mu(x)\log\frac{\mu(x)}{\nu(x)} \\
	&\ge \mu(A)\log\frac{\mu(A)}{\nu(A)}+\mu(X-A)\log\frac{\mu(X-A)}{\nu(X-A)}\\
	&\ge 2(\mu(A)-\nu(A))^2\\
	&= \frac{1}{2}\norm{\mu-\nu}{1}^2
	\end{align}
	\end{comment}
	\begin{align}
	\tilde{D}_C(\mu \parallel \nu) &= \sum_{x\in B}\mu(x)\log\frac{\mu(x)}{\nu(x)} + \sum_{x\in A-B}\mu(x)\log\frac{\mu(x)}{\nu(x)} + \sum_{x\in X-A}\mu(x)\log\frac{\mu(x)}{\nu(x)} \nonumber\\
	&= \delta\log C+ (p-\delta)\log\frac{p-\delta}{q-\epsilon}+(1-p)\log \frac{1-p}{1-q} \nonumber
	\end{align}
	\begin{enumerate}
		\item \emph{Case 1}: $\frac{\delta}{p} \ge 0.5$
		\begin{align}
		\tilde{D}_C(\mu \parallel \nu) &\ge \frac{p}{2}\log C +(1-p)\log \frac{1-p}{1-q}\nonumber \\
		&\ge 2(p-q)^2= \frac{1}{2}\norm{\mu-\nu}{1}^2 \nonumber
		\end{align}
		\item \emph{Case 2}: $\frac{\delta}{p} < 0.5$
		\begin{align}
		\tilde{D}_C(\mu \parallel \nu) &= \delta\log C+ (p-\delta)\log\frac{p}{q-\epsilon}+(p-\delta)\log\Big(1-\frac{\delta}{p}\Big)+(1-p)\log \frac{1-p}{1-q}\nonumber \\
		&\ge \delta\log C+ (p-\delta)\log\frac{p}{q}-(p-\delta)\frac{2\delta}{p}+(1-p)\log \frac{1-p}{1-q} \nonumber\\
		&\ge \delta(\log C-2)+ (p-\delta)\log\frac{p}{q}+(1-p)\log \frac{1-p}{1-q}\nonumber 
		\end{align}
		\begin{enumerate}
			\item \emph{Sub-case 1}: $\log \frac{p}{q} \ge 6$
			\begin{align}
			\tilde{D}_C(\mu \parallel \nu) &\ge (p-\delta)\log\frac{p}{q}+(1-p)\log \frac{1-p}{1-q}\nonumber\\
			&\ge 3p+(1-p)\log \frac{1-p}{1-q} \nonumber\\
			&\ge 2(p-q)^2= \frac{1}{2}\norm{\mu-\nu}{1}^2 \nonumber
			\end{align}
			\item \emph{Sub-case 2}: $\log \frac{p}{q} < 6$
			\begin{align}
			\tilde{D}_C(\mu \parallel \nu) &\ge \delta(\log C-2-\log\frac{p}{q})+ p\log\frac{p}{q}+(1-p)\log \frac{1-p}{1-q}\nonumber \\
			&\ge 2(p-q)^2= \frac{1}{2}\norm{\mu-\nu}{1}^2\nonumber
			\end{align}
		\end{enumerate}
	\end{enumerate}
\end{proof}
